# Supplementary material for: UniExtreme: A Universal Foundation Model for Extreme Weather Forecasting
Source: arXiv:2508.01426 source file (2025-09-04)
Supplement: Supplementary file 1 [file raw_var_appendix.tex]

\clearpage
                
\begin{table*}[ht]
\centering
\caption{Raw weather forecasting results for variable MSL. Gen. and Ext. indicate "General" and "Extreme".}
\resizebox{\linewidth}{!}{
% [inline block 0: 69 envs, 172861 chars -> data_tex | \begin{tabular}{c|ccc|ccc|ccc|ccc} \toprule...]

}
\label{table:raw_z_1000}
\end{table*}
